# Supplementary material for: U-Statistics for Importance-Weighted Variational Inference
Source: arXiv:2302.13918 source file (2023-02-27)
Supplement: Supplementary file 1 [file appendix-approximation.tex]

% Sections in aistats need to be all uppercase
\section{{Additional proofs regarding numerical approximations.}}
